# Supplementary material for: Approximate Modeling for Supercritical Galton-Watson Branching Processes with Compound Poisson-Gamma Distribution
Source: arXiv:2509.15502 source file (2025-10-17)
Supplement: Supplementary file 1 [file Supplemental_Material.pdf]

# Supplemental Material for “Approximate Modeling for Supercritical Galton–Watson Branching Processes with Compound Poisson–Gamma Distribution”

Kyoya Uemura  
Tomoyuki Obuchi  
Toshiyuki Tanaka

Department of Informatics, Graduate School of Informatics, Kyoto University, Kyoto 606-8501, Japan.

## S1 Alternative Derivation of the Approximate Solution $\tilde{K}(t)$

In this section, we show an alternative derivation of the approximate solution  $\tilde{K}(t)$ , given as (23) in the main paper, of the functional equation

$$\tilde{K}(\lambda t) = \psi(\tilde{K}(t)). \quad (12)$$

For the analysis below, we impose the following assumptions, which are the same as those that appeared in Sec. IV C.

### Assumption 1.

- (i) The offspring distribution is parameterized by its mean  $\lambda$ .
- (ii) The cumulant generating function

$$\psi(t) = \sum_{v=1}^{\infty} \frac{\kappa_v}{v!} t^v \quad (S1)$$

of the offspring distribution exists, where  $\kappa_v$  denotes the  $v$ th cumulant of the offspring distribution and  $\kappa_1 = \lambda$ .

(iii)  $\lim_{\lambda \downarrow 1} \kappa_2 = \kappa_2^* \in (0, \infty)$ .

(iv) For any  $\nu \geq 3$ , the order of the  $\nu$ th cumulant  $\kappa_\nu$  is  $o(1/(\lambda - 1)^{\nu-2})$  in the limit  $\lambda \downarrow 1$ .

Note that these assumptions are weaker than those in Sec. II A and concerns only the offspring distribution. It should also be noted that according to [1, Proposition 3], the moment generating function  $M_W(t)$  of  $W$  exists if Assumption 1-(ii) holds.

**Proposition S1.** Assume Assumption 1. For  $\lambda > 1$ , the power series expansion

$$\bar{K}(t) = \sum_{k=1}^{\infty} \frac{\bar{\kappa}_k}{k!} t^k \quad (\text{S2})$$

of the solution  $\bar{K}(t)$  of the functional equation (12) with  $\bar{\kappa}_1 = \lambda - 1$  is given in the asymptotic regime  $\lambda \downarrow 1$  by

$$\bar{\kappa}_k = k! \left( \frac{\kappa_2^*}{2} \right)^{k-1} (\lambda - 1) + o(\lambda - 1). \quad (\text{S3})$$

*Proof.* We prove (S3) via induction on  $k$ .

As one has  $\bar{\kappa}_1 = \lambda - 1$ , (S3) trivially holds for  $k = 1$ .

Substituting (S2) into (12), expanding both sides into power series in  $t$ , and comparing the coefficients of  $t^2$ -proportional terms, one has

$$\frac{1}{2} \lambda^2 \bar{\kappa}_2 = \frac{1}{2} \lambda \bar{\kappa}_2 + \frac{1}{2} \kappa_2 \bar{\kappa}_1^2,$$

which is simplified to

$$\frac{\bar{\kappa}_2}{\lambda - 1} = \frac{\kappa_2}{\lambda}. \quad (\text{S4})$$

From Assumption 1-(iii), the right-hand side of the above equation converges to  $\kappa_2^*$  in the limit  $\lambda \downarrow 1$ , showing that (S3) holds for  $k = 2$ .

Assume that (S3) holds for all  $l \in \{1, 2, \dots, k-1\}$  for  $k \geq 3$ . As above, substituting (S2) into (12), expanding both sides into power series in  $t$ , and comparing the coefficients of  $t^k$ -proportional terms, one has

$$\frac{\lambda}{k!} (\lambda^{k-1} - 1) \bar{\kappa}_k = \frac{\kappa_2}{2} \sum_{l=1}^{k-1} \frac{\bar{\kappa}_l}{l!} \frac{\bar{\kappa}_{k-l}}{(k-l)!} + (*). \quad (\text{S5})$$

The part  $(*)$  on the right-hand side of (S5) is a linear combination of terms of the form  $\kappa_\nu \prod_{j=1}^{\nu} \bar{\kappa}_{i_j}$ , where  $3 \leq \nu \leq k$ ,  $\sum_{j=1}^{\nu} i_j = k$ , and  $1 \leq i_j \leq k - \nu + 1$ . From (S5) one immediately has

$$\frac{\bar{\kappa}_k}{\lambda - 1} = \frac{1}{(\lambda - 1)^2 \sum_{l=1}^{k-1} \lambda^l} \left\{ \frac{\kappa_2}{2} \sum_{l=1}^{k-1} \binom{k}{l} \bar{\kappa}_l \bar{\kappa}_{k-l} + (*) \right\}. \quad (\text{S6})$$

For the first term on the right-hand side of (S6), one has, as  $\lambda \downarrow 1$ ,

$$\begin{aligned} \frac{1}{(\lambda-1)^2 \sum_{l=1}^{k-1} \lambda^l} \frac{\kappa_2}{2} \sum_{l=1}^{k-1} \binom{k}{l} \bar{\kappa}_l \bar{\kappa}_{k-l} &= \frac{\kappa_2}{2 \sum_{l=1}^{k-1} \lambda^l} \sum_{l=1}^{k-1} k! \left( \frac{\kappa_2^*}{2} \right)^{k-2} + o(1) \\ &= k! \left( \frac{\kappa_2^*}{2} \right)^{k-1} + o(1), \end{aligned} \quad (\text{S7})$$

where the second line is derived from the inductive hypothesis, that is, (S3) for  $l \in \{1, 2, \dots, k-1\}$ .

We next investigate the part  $(*)$  on the right-hand side of (S6) in the limit  $\lambda \downarrow 1$ . As mentioned above, the part  $(*)$  is a linear combination of terms of the form  $\kappa_\nu \prod_{j=1}^\nu \bar{\kappa}_{i_j}$  with  $\nu \geq 3$ . From the inductive hypothesis and Assumption 1-(iv), for  $\nu \geq 3$ ,

$$\begin{aligned} \frac{1}{(\lambda-1)^2} \times \kappa_\nu \prod_{j=1}^\nu \bar{\kappa}_{i_j} &= (\lambda-1)^{\nu-2} \kappa_\nu \prod_{j=1}^\nu \frac{\bar{\kappa}_{i_j}}{\lambda-1} \\ &= (\lambda-1)^{\nu-2} \kappa_\nu \left( \prod_{j=1}^\nu i_j! \left( \frac{\kappa_2^*}{2} \right)^{i_j-1} + o(1) \right) \\ &= o(1). \end{aligned} \quad (\text{S8})$$

One therefore obtains

$$\frac{1}{(\lambda-1)^2 \sum_{l=1}^{k-1} \lambda^l} \times (*) = o(1) \quad (\text{S9})$$

From these results, the right-hand side of (S6) is equal to

$$k! \left( \frac{\kappa_2^*}{2} \right)^{k-1} + o(1) \quad (\text{S10})$$

as  $\lambda \downarrow 1$ . We have therefore shown that (S3) holds for  $k$ .

Via induction, we have proved the proposition.  $\square$

Let

$$\tilde{\kappa}_k = k! \left( \frac{\kappa_2^*}{2} \right)^{k-1} (\lambda-1) \quad (\text{S11})$$

be the leading-order term of (S3). It is then straightforward to confirm that the following cumulant generating function

$$\tilde{K}(t) = \frac{(\lambda-1)t}{1 - \frac{\kappa_2^* t}{2}} \quad (23)$$

has the  $k$ th cumulant equal to  $\tilde{\kappa}_k$  for any  $k$ . This coincides with the result obtained via the perturbative analysis in Sec. II-A.

## S2 Extinction probabilities of the GW model and the CPG model

### S2.1 The Poisson offspring distribution

The probability  $\mathbb{P}(W = 0)$  of the limiting distribution of the GW process (referred to as the *extinction probability*) is generally given as the smallest root of  $f(s) = s$  for  $s \in [0, 1]$  [2]. By solving the equation  $f(s) = s$  with the Poisson probability generating function, the extinction probability  $\mathbb{P}(W = 0)$  for the supercritical case  $\lambda > 1$  is obtained as

$$\mathbb{P}(W = 0) = -\frac{W_0(-\lambda e^{-\lambda})}{\lambda}, \quad (\text{S12})$$

where  $W_0(\cdot)$  denotes the principal branch of the Lambert  $W$  function.

On the other hand, the probability  $P_{\text{CPG}}(0; \mu, \alpha, \tau)$  of the CPG distribution at zero is given as the probability of its Poisson random variable  $N$  being equal to 0, i.e.,

$$P_{\text{CPG}}(0; \mu, \alpha, \tau) = \mathbb{P}(N = 0) = e^{-\mu}. \quad (\text{S13})$$

In the case of the Poisson offspring distribution, one has  $\kappa_2^* = 1$ , so that one obtains, from (S13) and (30),

$$P_{\text{CPG}}\left(0; \frac{2(\lambda - 1)}{\kappa_2^*}, 1, \frac{\kappa_2^*}{2(\lambda - 1)}\right) = \exp\{-2(\lambda - 1)\}. \quad (\text{S14})$$

Hence,

$$\begin{aligned} \mathbb{P}(W = 0) - P_{\text{CPG}}\left(0; \frac{2(\lambda - 1)}{\kappa_2^*}, 1, \frac{\kappa_2^*}{2(\lambda - 1)}\right) &= -\frac{W_0(-\lambda e^{-\lambda})}{\lambda} - \exp\{-2(\lambda - 1)\} \\ &= \exp\left\{-W_0(-\lambda e^{-\lambda}) - \lambda\right\} - \exp\{-2(\lambda - 1)\} \\ &= e^{-2(\lambda - 1)} \left[ \exp\left\{\lambda - 2 - W_0(-\lambda e^{-\lambda})\right\} - 1 \right]. \end{aligned} \quad (\text{S15})$$

We now claim the inequality

$$(\lambda - 2)e^{\lambda - 2} > -\lambda e^{-\lambda}, \quad \forall \lambda > 1, \quad (\text{S16})$$

to hold. Once we admit it, one has

$$W_0\left((\lambda - 2)e^{\lambda - 2}\right) > W_0\left(-\lambda e^{-\lambda}\right) \quad (\text{S17})$$

because  $W_0(x)$  is monotonically increasing for  $x > -1/e$ . The left-hand side of the above inequality is equal to  $\lambda - 2$  by the definition of  $W_0$ , so that one obtains

$$\lambda - 2 > W_0(-\lambda e^{-\lambda}), \quad (\text{S18})$$

which shows that (S15) is positive, thus proving

$$\mathbb{P}(W = 0) > P_{\text{CPG}}\left(0; \frac{2(\lambda - 1)}{\kappa_2^*}, 1, \frac{\kappa_2^*}{2(\lambda - 1)}\right) \quad (\text{S19})$$

to hold for any  $\lambda > 1$ .

What remains is to prove the inequality (S16). We start with the inequality

$$x > \tanh x = \frac{e^x - e^{-x}}{e^x + e^{-x}}, \quad \forall x > 0, \quad (\text{S20})$$

which can be rearranged as

$$(x - 1)e^{x-1} > -(x + 1)e^{-(x+1)}. \quad (\text{S21})$$

Substituting  $x = \lambda - 1 > 0$  into (S21) proves (S16).

The result (S19) means that the approximation with the CPG model (30) always underestimates the extinction probability of the supercritical GW process with the Poisson offspring distribution.

## S2.2 The geometric offspring distribution

As in the preceding subsection, one can evaluate the extinction probability  $\mathbb{P}(W = 0)$  with the geometric offspring distribution

$$P_{\text{geo}}(x) = p(1 - p)^x, \quad x \in \{0, 1, 2, \dots\}, \quad (\text{S22})$$

and the corresponding probability  $P_{\text{CPG}}(0; \mu, \alpha, \tau)$  of the CPG distribution at zero.

Using the fact that the geometric offspring distribution  $P_{\text{geo}}(x)$  has the moment generating function  $f(s) = 1/(1 + \lambda - \lambda s)$  with the mean  $\lambda = (1 - p)/p > 1$ , one can find the solution of the equation  $f(s) = s$  with  $s < 1$  to obtain the extinction probability  $\mathbb{P}(W = 0)$  as

$$\mathbb{P}(W = 0) = \frac{p}{1 - p} = \frac{1}{\lambda}. \quad (\text{S23})$$

On the other hand, from the variance  $\kappa_2 = \frac{1-p}{p^2}$  of the geometric distribution, one has

$$\kappa_2^* = \lim_{\lambda \downarrow 1} \frac{1-p}{p^2} = \lim_{\lambda \downarrow 1} \lambda^2 + \lambda = 2. \quad (\text{S24})$$

Hence, from (S13) and (30), one obtains

$$P_{\text{CPG}} \left( 0; \frac{2(\lambda-1)}{\kappa_2^*}, 1, \frac{\kappa_2^*}{2(\lambda-1)} \right) = \exp\{-(\lambda-1)\}. \quad (\text{S25})$$

For  $\lambda > 1$ , one has the inequality  $e\lambda < e^\lambda$ , which is rearranged as

$$\frac{1}{\lambda} > \exp\{-(\lambda-1)\}. \quad (\text{S26})$$

The above inequality, along with (S23) and (S25), implies the relation

$$\mathbb{P}(W=0) > P_{\text{CPG}} \left( 0; \frac{2(\lambda-1)}{\kappa_2^*}, 1, \frac{\kappa_2^*}{2(\lambda-1)} \right). \quad (\text{S27})$$

Thus, the approximation with the CPG model underestimates the extinction probability of the limiting distribution in the case of the geometric offspring distribution as well.

## References

- [1] J. D. Biggins and D. N. Shanbhag, “Some divisibility problems in branching processes,” *Mathematical Proceedings of the Cambridge Philosophical Society*, vol. 90, no. 2, pp. 321–330, 1981.
- [2] K. B. Athreya and P. E. Ney, *Branching Processes*. Springer Berlin, 1972.
